# Supplementary material for: Generalized Deployable Elastic Geodesic Grids
Source: arXiv:2111.08883 source file (2021-11-17)

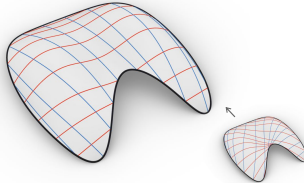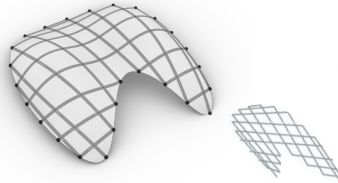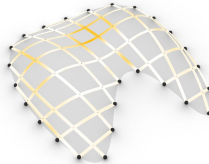

0 [cm]

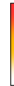

0.5 [cm]

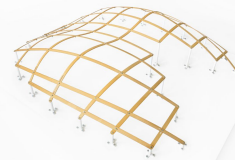

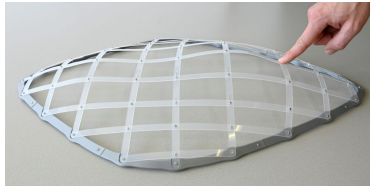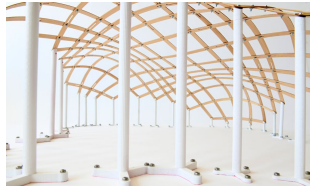

Supplement: Supplementary file 1 [file result_additional_v5.pdf]
